# Supplementary material for: Operational Aspects of C/C++ Concurrency
Source: arXiv:1606.01400 source file (2016-07-09)
Supplement: Supplementary file 1 [file appendix.tex]

\section{Intuition and [Batty-al:POPL11]}

\subsection{Happens-Before}
The main difference of weak memory models to sequential consistent ones is that
there is no total order on memory operations for program executions.
Or it is better to say,
that an observation order on actions is \emph{subjective} for threads.
Consider an example on Fig.\ref{fig:iriw}. There is a valid execution in
a C11 memory model that ends with \texttt{r0 = r2 = 1}, \texttt{r1 = r3 = 0}.
It means, that the third thread observed \texttt{x = 1} before \texttt{y = 1}, and
the fourth thread observed them in a reverse order. But both of threads have to observed 
\texttt{x = 0; y = 0} before \texttt{x = 1} and \texttt{y = 1}. 
Thus still there are some relations, which restrict the observation order.

\begin{wrapfigure}[5]{r}[0pt]{0.55\textwidth} 
\centering 
\begin{tabular}{l@{\ \ \ }l}
\begin{minipage}[l]{4.7cm}
\small
\begin{verbatim}
          x = 0; y = 0
x = 1 || y = 1 || r0 = x || r2 = y
      ||       || r1 = y || r3 = x
\end{verbatim} 
\end{minipage}
&
\end{tabular}
\caption{The IRIW example.}
\label{fig:iriw}
\end{wrapfigure}

To formally introduce these relations we need to outline some basic notions and ideas of
an axiomatic semantics for C11 \cite{Batty-al:POPL11}. This semantics 
represents a C11 program execution as a graph with nodes denoted to \emph{memory actions}
and edges representing different relations between memory actions.
Every memory action can be either \emph{read}, \emph{write} or \emph{read-modify-write} (RMW).
In the rest of a paper then we speak about read actions in general we also assume RMW actions
if we don't state the opposite explicitly. The same is true for write and RMW actions.
A memory action has a number of attributes. First, it is labeled by
a location, which it operates on. Second, it has a value.
If the action is read one then it is the value, which is read from the location by the action.
And if the action is write one then it is the value written to the location.
Third, the memory action is labeled by a \emph{memory order},
which can be \emph{relaxed}, \emph{release}, \emph{acquire}, \emph{sc}, \emph{consume},
\emph{acquire\_release}, or \emph{non-atomic}.

\app{TODO: put here a lattice of modificators}

\app{TODO: put here a graph example}

%\begin{wrapfigure}{l}{\textwidth}
%\input{iriw}
%\end{wrapfigure}

In any valid execution graph every read action has to be connected
with one and only one write action to a same location by a \readFrom~edge (\emph{rf}).
It means that the read action `reads' a value that was written by the write action. 
An edge with \readFrom~label can be also a part of a \synchronizedWith~relation, if it 
connects a \emph{release} write with an \emph{acquire} read. 

An another important relation is \programOrder.
It connects memory actions of a same thread in natural order of their execution, as they
are executed in a single thread case.
We should notice that this order can't be determined statically in case of
C and C++ languages, because of constructions like \texttt{==} operator, for which the
language standards don't determine an order on its arguments computation.
Beside, every first action of every thread is connected by \asw~edge with an parent thread
action, which is the last
\programOrder-before the thread spawn.

In a C11 subset without \emph{consume} actions a transitive closure of \synchronizedWith~and
\programOrder~is a \happensBefore~relation. It is the most important relation in the model.
It is a generalization of total order of sequential consistent models mentioned above.
Thus the \happensBefore~relation 
means that a later in \happensBefore~sense action has to observe a result of an earlier one.
And this relation restricts a \readFrom~relation in a natural way --- a read action can't be connected
with a write action by a \readFrom~edge, if it is \happensBefore~than the write one.
An intuition behind this restriction is than the read action can't `read' from its future.

\subsection{Location Atomicity}
In C11 (as a language, not a memory model)
a variable can be either \emph{atomic} or \emph{non-atomic} one. An atomic variable has
an special type \texttt{atomic<*>} (\eg \texttt{atomic<int>}, \texttt{atomic<bool>}), and
it can be operated with all memory modifiers except \emph{non-atomic} one. An non-atomic variable
has a plain type (\eg \texttt{int}, \texttt{bool}, \texttt{string}), and only 
memory operations with \emph{non-atomic} modificator can used to operate on it.

It is important to notice that we previously described the C11 memory model in terms of locations,
not variables. Beside, in real C/C++ one can cast an atomic variable to a plain type and start operate
on it using non-atomic operations.

\subsection{Memory-order}
An other relation in the semantics of C11 is a \memoryOrder. It totally orders write actions
to a same location, beside that it is consistent with the \happensBefore~relation.
It is worth to note that if a program in the C11 memory model manipulates only one location,
then it has a same behaviour as in a sequential consistent model\footnote{But it is true only for atomic
locations, because data races on non-atomic locations still lead to undefined behaviour}.

In our semantics we don't distinguish non-atomic and atomic locations, and every
location can be manipulated by non-atomic and atomic operations. But our semantics identifies
data races on non-atomic operations.
